# Supplementary material for: Deep Backtracking Counterfactuals for Causally Compliant Explanations
Source: arXiv:2310.07665 source file (2024-08-10)
Supplement: Supplementary file 1 [file suppl_visualizations_celeba.pdf]

(a)

*“What would have been, had this person been ...*

(i)

factual

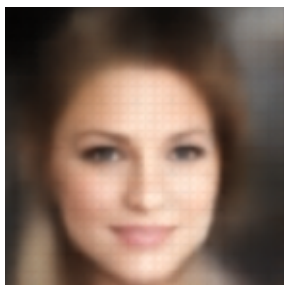

*... old?”*

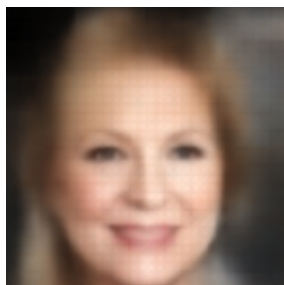

*... old and male?”*

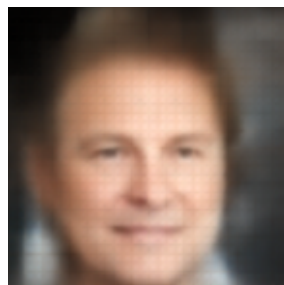

(ii)

factual

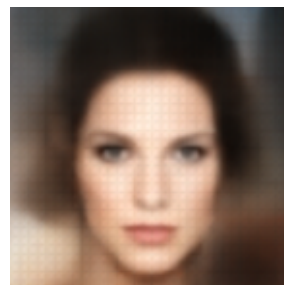

*... male?”*

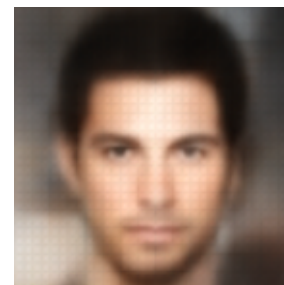

*... male and bearded?”*

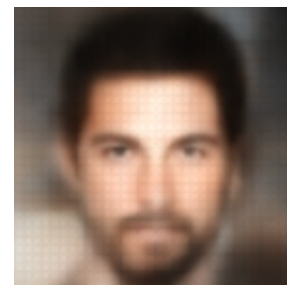

(b)

*“What would have been, had this person not had a beard?”*

factual

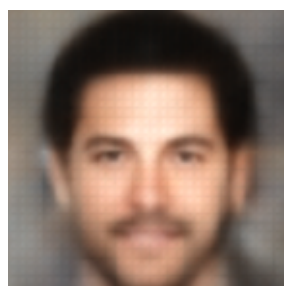

DeepBC

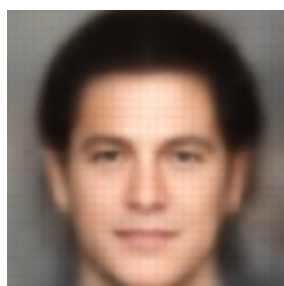

interventional

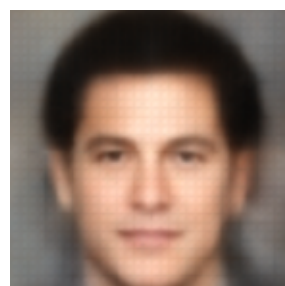

tabular explanation

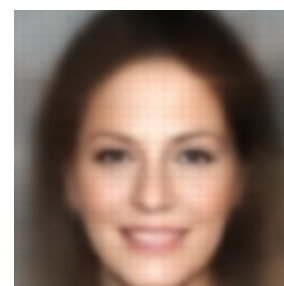

(c)

*“What would have been, had this person been bearded?”*

factual

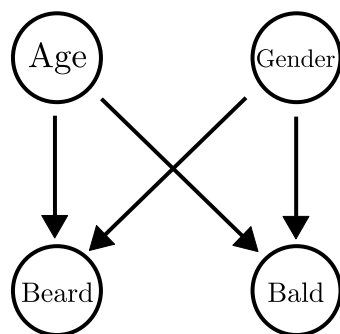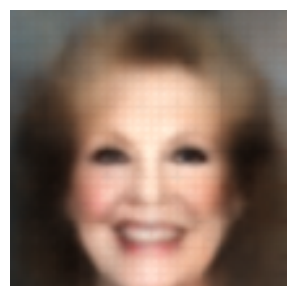

sparse DeepBC

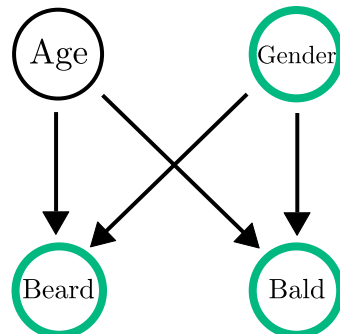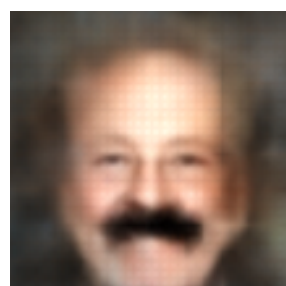

sparse DeepBC  
w. wrong graph

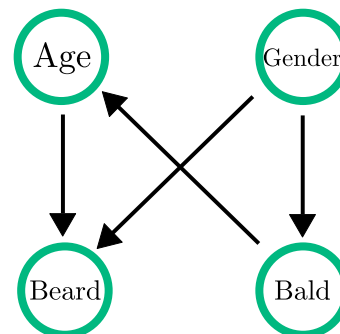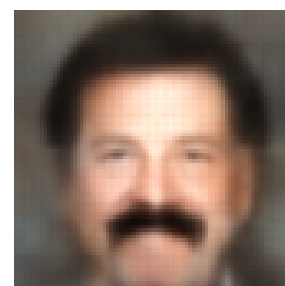

?”
